# Supplementary material for: VoxGRAF: Fast 3D-Aware Image Synthesis with Sparse Voxel Grids
Source: arXiv:2206.07695 source file (2022-11-09)
Supplement: Supplementary file 1 [file appendix.tex]

\clearpage
\begin{eqnarray}
Var(z) &=& \sum_k w_k (z-z_k)^2\\
\frac{d}{d\sigma_i}Var(z) &=& \sum_k \left[ \frac{dw_k}{d\sigma_i} (z-z_k)^2 +  w_k  \frac{d(z-z_k)^2}{d\sigma_i} \right] \\
&=& \sum_k \left[ \frac{dw_k}{d\sigma_i} (z-z_k)^2 +  w_k  \frac{d(z-z_k)^2}{dz}\frac{dz}{d\sigma_i} \right]\\
\sum_k \frac{dw_k}{d\sigma_i} C_k &=& \frac{dw_i}{d\sigma_i} C_i + \sum_{k>i}C_k \frac{dw_k}{d\sigma_i}\\
&=&\delta_i\left[C_iT_i - \sum_{k\geq i} C_k w_k\right] \\
\sum_k w_k  \frac{d(z-z_k)^2}{dz}\frac{dz}{d\sigma_i} &=& 2\frac{z}{d\sigma_i}\sum_k w_k(z-z_k)
\end{eqnarray}

\clearpage

\begin{itemize}
    \item spherical harmonics
    \item skip architecture
    \item sigma multiplier
    \item carla - sparsity loss?
    \item pose conditioning -> use 12 dim vector containing RT
    \item uncurated samples
    \item lazy reg
    \item failure cases
    \item value of $\tau$ for depth variance loss
    \item societal impact
    \item BG/FG disentanglement
\end{itemize}

We can make the following choices
\begin{itemize}
    \item $z^{fg} = z^{bg}$ or $z^{fg} \neq z^{bg}$ (shared latent or independent fg/bg)
    \item $G_m^{bg}(z^{bg})$ or $G_m^{bg}(z^{bg}, \xi_\bI)$ (static background or conditioned on pose)
    \item $\xi_\bI \sim p_D$ or $\xi_\bI \sim \mathcal{U}(\xi_{min}, \xi_{max})$ (sample from data distribution or uniform pose sampling)
\end{itemize}

\boldparagraph{Sparsity Loss (3D)}
To encourage a high sparsity of the generated voxel grid we can impose several regularizers.
Plenoxels~\cite{Yu2021cARXIV} propose a sparsity loss
\begin{align}
    \cL_s = \lambda_s \sum_{i}^{R_G^3}\log (1+2\sigma_i^2)
\end{align}
which encourages the densities of all voxels to be close to zero.

\boldparagraph{Binary Loss (2D)}
Plenoxels further encourages $\hat{\bI}^{fg}_{mask}$ to take values close to zero or one with a beta loss
\begin{align}
    \cL_{\beta_{2D}} = \lambda_{\beta_{2D}} \log(T^{fg}(\br)) + \log(1-T^{fg}(\br))
\end{align}
where $T^{fg}$ is the accumulated transmittance along ray $\br$, i.e. $T^{fg}(\br)=\exp(\sum_i^{N-1}-\sigma_i\delta_i)$.\\
A similar loss is used in GIRAFFE-HD~\cite{Xue2022CVPR}, but is applied to the mask instead of the accumulated transmittance.
Further, GIRAFFE-HD~\cite{Xue2022CVPR} directly regularizes the masks to cover at least some fraction $\eta$ of the image
\begin{align}
    \cL_{cvg} = \max(\eta, \frac{1}{|\cS|}\sum_{i\in\cS} \min( \hat{\bI}^{fg}_{mask}[i], 1-\hat{\bI}^{fg}_{mask}[i])
\end{align}
which we can use for both, foreground and background.

\boldparagraph{Binary Loss (3D)}
We remark that this rendering-based on-the-fly pruning becomes computationally feasible through the use of custom CUDA kernels.

Plenoxels directly optimizes the grid values for a single instance. To reduce computation, they use a sigma threshold during rendering which avoids computing values for voxels inside the object.
Instead, we generate different voxel grids for all instances. Hence, we benefit from generating \textit{hollow} voxel grids with sparse convolutions. Hence, we need a regularizer that encourages voxels inside the object to be empty.
Instead of using a 3D sparsity loss and a 2D beta loss, we directly regularize the voxel densities to make the voxel either empty or fully opaque
\begin{align}
    \cL_{3D}  = \lambda_{3D} \left( \sum_{\bv\in\cV_r} ||\ |\sigma(\bv)| - \sigma^*||_2
     + \sum_{\bv\notin\cV_r} ||\sigma(\bv) - (-\sigma^*)||_2 
    \right)
\end{align}
where $\cV_r$ denotes the set of rendered voxels using some sigma threshold for stopping and $\sigma^*$ is some target value for the density.
In practice, we slowly increase $\sigma^*$ during training until voxels are fully opaque.
Note, that this is somewhat similar to~\cite{Xu2021NEURIPS}, which impose a 3D beta loss on the predicted opacities $\alpha_i=1-\exp(\sigma_i\delta_i)$. However, their generator directly predicts opacities instead of densities and does not differ between rendered and non-rendered voxels.

\boldparagraph{Depth Variance}
\begin{align}
    \hat{z} = \sum_i T_i\alpha_i z_i\\
    var(\hat{z}) = \sum_i T_i\alpha_i (z_i-\hat{z})^2\\
    \cL_{var(\hat{z})} = \lambda_{var(\hat{z})} var(\hat{z})
\end{align}

\boldparagraph{Smoothness Loss (2D)}
To encourage compactness of the voxel grid, we could directly regularize the rendered depth to be smooth
\begin{align}
    \cL_{TV_{2D}} = \lambda_{TV_{2D}} \frac{1}{|\cP|} \sum_{\bp\in\cP}\sqrt{\Delta^2_x(\bp)+\Delta^2_y(\bp)}
\end{align}
where $\cP$ denotes the set of pixels in the rendered depth map.

\boldparagraph{Smoothness Loss (3D)}
Instead, Plenoxels encourages a compact voxel grid to by regularizing its total variation
\begin{align}
    \cL_{TV} = \lambda_{TV} \frac{1}{|\cV|} \sum_{\bv\in\cV, d\in[D]}\sqrt{\Delta^2_x(\bv, d)+\Delta^2_y(\bv, d)+\Delta^2_z(\bv, d)}
\end{align}
with $\Delta^2_x(\bv, d)$ shorthand for the squared difference between the $d$-th value in voxel $v := (i, j, k)$ and the  $d$-th value in voxel $(i + 1, j, k)$ normalized by the resolution, and analogously for $\Delta^2_y(\bv, d)$ and $\Delta^2_z(\bv, d)$.

\boldparagraph{Total Variation Loss}
Without regularization, volume rendering is prone to result in semi-opaque voxels and floating artifacts and struggles to accurately represent sharp surfaces~\cite{Niemeyer2021CVPR,Jain2021CVPR,Oechsle2019ICCV,Xu2021NEURIPS}.
Following Plenoxels~\cite{Yu2021cARXIV}, we regularize the total variation of the predicted density values in the set of all voxels $\cV$ for a compact, smooth geometry
\begin{align}
    \cL_{TV} = \lambda_{TV} \frac{1}{|\cV|} \sum_{\bv\in\cV}\sqrt{\Delta^2_x(\sigma)+\Delta^2_y(\sigma)+\Delta^2_z(\sigma)}
\end{align}
with $\Delta^2_x(\sigma)$ shorthand for $(\sigma_{i,j,k}-\sigma_{i+1,j,k})^2$ and analogously for $\Delta^2_y(\sigma)$ and $\Delta^2_z(\sigma)$. \michael{moved from the main paper to here}

\boldparagraph{Mask Coverage Loss}
To avoid that the full image is generated by either background or foreground generator, we use a hinge loss on the
mean mask value as proposed in  GIRAFFE-HD~\cite{Xue2022CVPR}
\begin{eqnarray}
    \cL_{cvg}^{fg} &=& \max\left(0, \eta^{fg}-\frac{1}{|\cS|}\sum_{i\in\cS} \hat{\bI}^{fg}_{mask}[i]\right)\\
    \cL_{cvg}^{bg} &=& \max\left(0, \eta^{bg}-\frac{1}{|\cS|}\sum_{i\in\cS} 1-\hat{\bI}^{fg}_{mask}[i]\right)
\end{eqnarray}
where $\eta^{fg}$ and $\eta^{bg}$ denote the minimum fraction that should be covered by foreground and background, respectively. To ensure that both models are used, we find that roughly \michael{what does roughly mean? You cannot set the value to roughly something, no?} setting $\eta^{fg}=0.4$ and $\eta^{bg}=0.1$ is sufficient. \michael{moved from the main paper to here}

\clearpage

\subsection{VoxGRAF: Generating Explicit Scence Representations}

Instead of representing the scene implicitly, our approach generates an \textit{explicit} sparse voxel grid. The voxel grid is synthesized by a 3D generator $G_\theta$, which only receives a latent $\bz$ as input.
This formulation is in contrast to implicit approaches employing MLPs conditioned on a latent, coordinates, and viewing direction.
Following Yu et~al.~\cite{Yu2021cARXIV}, we compute $(\sigma_r^i,\bc_r^i)$ via trilinear interpolation of densities and colors stored at the nearest eight voxels.
We use the same rendering formulation outlined in~\ref{subsec:implicit_gan} and leverage custom CUDA kernels\footnote{\url{https://github.com/sxyu/svox2.git}} for efficiency.

There are several choices for designing the 3D generator.
The generator may use 2D or 3D convolutions to generate density values $\mathbf\sigma\in\mathbb{R}^{1\times R_G\times R_G\times R_G}$ and color values $\bc\in\mathbb{R}^{3\times R_G\times R_G\times R_G}$ on a 3D grid with resolution $R_G$.
A 2D CNN needs to be followed by a reshape operation, whereas a 3D CNN generates a 3D grid directly.
While 2D convolutions can leverage established 2D CNN generators, 3D convolutions potentially allow for better 3D modeling because they maintain a 3D structure. Further, the 3D structure makes the representation suitable for pruning and applying sparse operations.
As our focus is 3D-consistency, the generator does not model view-dependent effects.

All architectures build on the StyleGAN2 generator~\cite{Karras2019CVPR}, as it achieves high fidelity in the 2D domain and provides fine-grained semantic control.
The StyleGAN2 generator consists of a mapping network $\mathbf{G}_m$ and a synthesis network $\mathbf{G}_s$.
First, $\mathbf{G}_m$ maps a latent code $\bz\in\mathcal{N}(0, 1)$ to a style code
$\mathbf{w}$. $\mathbf{w}$ is then used to modulate the convolution kernels of $\mathbf{G}_s$ to control the synthesis process of a 2D image.
We outline the possible designs below and visualize them in \figref{fig:generators}.
\generators

\boldparagraph{2D CNN + Pixelshuffle.}
$G_\theta$ generates a 2D feature map $\bF\in\mathbb{R}^{d_f\times R_G\times R_G}$, where the channel dimension $d_f=4 R_G$.
The feature map is converted to color and density values on a 3D grid via Pixelshuffle~\cite{Shi2016CVPRa}.
Concretely, we rearrange the channel dimension $d_f$ into an additional spatial dimension and $3+1$ channels for color and density, respectively, yielding a voxel grid of size $\mathbb{R}^{4 \times R_G\times R_G\times R_G}$.

\boldparagraph{2D CNN + Multi-Plane Decoder.} 
Similar to~\cite{Peng2020ECCV}, $G_\theta$ generates three canonical planes $\mathbf{XY}$, $\mathbf{XZ}$, $\mathbf{YZ}$ $\in\mathbb{R}^{4\times H\times W}$ by splitting the generated 2D feature map $\mathbf{F}\in\mathbb{R}^{4\cdot3\times H\times W}$ along the channel dimension. 
We aggregate the color and density values at grid position $(i,j,k)$ using summation and an orthographic projection.
\begin{align}
   (\mathbf{\sigma}_{ijk},\mathbf{c}_{ijk}) = \mathbf{XY}_{ij} + \mathbf{XZ}_{ik}  + \mathbf{YZ}_{jk} 
\end{align}

\boldparagraph{3D CNN.}
We replace all 2D operations of the StyleGAN2 generator $\mathbf{G}_\theta$ with their 3D equivalent, e.g., 3D modulated convolutions and 3D upsampling. $\mathbf{G}_\theta$ directly generates the voxel grid of size $\mathbb{R}^{4 \times R_G\times R_G\times R_G}$.
We compare between a fully dense generator (3D dense) and a generator employing sparse convolution~\cite{Choy2019CVPR} (3D sparse).

Sparse convolutions are advantageous over dense ones as they are more computationally efficient. We observe no additional benefit from sparse convolutions at smaller resolutions. Hence, we keep a dense representation until a resolution of $32^3$ and use sparse convolutions beyond.
To sparsify the representation, we combine progressive growing~\cite{Karras2018ICLR} with weight-based pruning~\cite{Yu2021cARXIV}.
Specifically, we start training a dense model on resolution $32^3$. When sufficiently trained, we prune its output based on the generated density $\mathbf{\sigma}$. We follow~\cite{Yu2021cARXIV} and prune voxels with $\mathbf{\sigma}\le0$  if the same also holds for their neighbors. We then add layers for the subsequent higher resolution, which receive the pruned feature grid as input.

\boldparagraph{Ablation.}
We conduct an ablation on CARLA~\cite{Schwarz2020NEURIPS} at resolution $512^2$ to compare the generator architectures.
\tabref{tab:ablation} reports the results on CARLA at resolution $512^2$.
\red{Fill with results.}
 
\ablation

\subsection{Baseline Implementations}

Describe that we use the official codes with links\footnote{\url{https://github.com/marcoamonteiro/pi-GAN.git}\\\url{https://github.com/SheldonTsui/GOF_NeurIPS2021.git}\\\url{https://github.com/facebookresearch/StyleNeRF.git}}

As proposed in~\cite{Chan2021ARXIV}, we report multi-view facial identity consistency (ID) using ~\cite{Deng2019CVPR} on FFHQ. We further analyze shape accuracy by computing the MSE against pseudo-ground-truth depth-maps on FFHQ~\cite{Deng2019CVPRWork,Shi2021CVPR}
