# Supplementary material for: VoxGRAF: Fast 3D-Aware Image Synthesis with Sparse Voxel Grids
Source: arXiv:2206.07695 source file (2022-11-09)
Supplement: Supplementary file 2 [file abstract.tex]

\begin{abstract}
In this \textbf{supplementary document}, 
we first provide details on the network architectures and training strategy of our approach in \secref{sec:supp_implementation}. Our settings for the baselines are described in \secref{sec:supp_baselines}.
\secref{sec:supp_results} shows additional results and failure cases.
In \secref{sec:supp_discussion}, we discuss the societal impact of our work. The \textbf{supplementary video} includes synthesized animations in which we control the camera viewpoint for our method and the baselines and show interpolations between latent codes. We use the same mathematical notation as in the paper.
\end{abstract}
